# Supplementary material for: Alexa as an Active Listener: How Backchanneling Can Elicit Self-Disclosure and Promote User Experience
Source: arXiv:2204.10191 source file (2022-09-22)
Supplement: Supplementary file 1 [file Survey_Measures.pdf]

## PRE—STUDY SURVEY:

### Demographics

Age Please indicate your age category.

- ○ 18-20 (1)
- ○ 21-24 (2)
- ○ 25-30 (3)
- ○ 31-34 (4)
- ○ 35-40 (5)
- ○ 41-50 (7)
- ○ older than 50 (8)

---

Gender What gender do you identify with?

- ○ Female (1)
- ○ Male (2)
- ○ Other (4)

---

Language Is English your native (first) language?

- ○ Yes (1)
- ○ No (2)

---

Relationship What is your marital status?

- ○ Married (1)
- ○ Single (2)
- ○ Divorced (3)
- ○ In a relationship (4)

---

School Which of the following categories best describes your education status?

- ○ College Student (1)
- ○ Graduate Student (2)
- ○ Post-graduate (3)
- ○ Never went to college (4)
- ○ College Almuni (5)

---

Prior Experience with smart speakers
Do you use any smart-speaker assistants such as Siri, Google home, or Alexa?

- ○ Yes, regularly (1)
- ○ Yes, but not often (2)
- ○ No (4)

**Pre- study emotional wellbeing, PANAS measures by Watson et al., 1988.**

On the scale of 1 (Not at All) to 10 (Very Much), how well do the following adjectives represent **how you feel at the moment**?

| | 1 (221) | 2 (222) | 3 (223) | 4 (224) | 5 (225) | 6 (226) | 7 (227) | 8 (228) | 9 (229) | 10 (230) |
|---|---|---|---|---|---|---|---|---|---|---|
| Enthusiastic (231) | ○ | ○ | ○ | ○ | ○ | ○ | ○ | ○ | ○ | ○ |
| Sad (232) | ○ | ○ | ○ | ○ | ○ | ○ | ○ | ○ | ○ | ○ |
| Content (233) | ○ | ○ | ○ | ○ | ○ | ○ | ○ | ○ | ○ | ○ |
| Embarrassed (234) | ○ | ○ | ○ | ○ | ○ | ○ | ○ | ○ | ○ | ○ |
| Nervous (235) | ○ | ○ | ○ | ○ | ○ | ○ | ○ | ○ | ○ | ○ |
| Angry (236) | ○ | ○ | ○ | ○ | ○ | ○ | ○ | ○ | ○ | ○ |
| Calm (237) | ○ | ○ | ○ | ○ | ○ | ○ | ○ | ○ | ○ | ○ |
| Anxious (238) | ○ | ○ | ○ | ○ | ○ | ○ | ○ | ○ | ○ | ○ |
| Happy (239) | ○ | ○ | ○ | ○ | ○ | ○ | ○ | ○ | ○ | ○ |
| Active (240) | ○ | ○ | ○ | ○ | ○ | ○ | ○ | ○ | ○ | ○ |

## POST—STUDY SURVEY:

**Emotional Effectiveness of Alexa, measures of effectiveness from Stiles et al., 2006.**

Effectiveness On the scale of 1 (Strongly Disagree) to 10 (Strongly Agree), please evaluate the extent to which you agree on the following statements about your interaction with Alexa.

| | 1 (1) | 2 (2) | 3 (3) | 4 (4) | 5 (5) | 6 (6) | 7 (7) | 8 (8) | 9 (9) | 10 (10) |
|---|---|---|---|---|---|---|---|---|---|---|
| I feel better after talking with Alexa (426) | ○ | ○ | ○ | ○ | ○ | ○ | ○ | ○ | ○ | ○ |
| After talking with the Alexa, I feel less depressed (427) | ○ | ○ | ○ | ○ | ○ | ○ | ○ | ○ | ○ | ○ |
| The way Alexa talked to me irritated me (428) | ○ | ○ | ○ | ○ | ○ | ○ | ○ | ○ | ○ | ○ |
| Talking with Alexa helped me get my mind off the negative experience (429) | ○ | ○ | ○ | ○ | ○ | ○ | ○ | ○ | ○ | ○ |
| Alexa made me feel better about myself (430) | ○ | ○ | ○ | ○ | ○ | ○ | ○ | ○ | ○ | ○ |
| I feel more optimistic after talking with Alexa (431) | ○ | ○ | ○ | ○ | ○ | ○ | ○ | ○ | ○ | ○ |

| | | | | | | | | | | |
|---|---|---|---|---|---|---|---|---|---|---|
| It helped me understand the situation better to talk it over with Alexa (432) | ○ | ○ | ○ | ○ | ○ | ○ | ○ | ○ | ○ | ○ |
| Alexa seemed really concerned about me (433) | ○ | ○ | ○ | ○ | ○ | ○ | ○ | ○ | ○ | ○ |
| Alexa’s responses were appropriate (434) | ○ | ○ | ○ | ○ | ○ | ○ | ○ | ○ | ○ | ○ |
| I felt that Alexa was putting me down (435) | ○ | ○ | ○ | ○ | ○ | ○ | ○ | ○ | ○ | ○ |
| I wish Alexa’s responses had been briefer (436) | ○ | ○ | ○ | ○ | ○ | ○ | ○ | ○ | ○ | ○ |
| I wish Alexa’s responses had been longer (437) | ○ | ○ | ○ | ○ | ○ | ○ | ○ | ○ | ○ | ○ |

**Perceived Active Listening, measure of active-empathetic listening by Gearhart, C.C., &Bodies, G.D., 2011.**

On the scale of 1 (Strongly Disagree) to 10 (Strongly Agree), please evaluate the extent to which you agree on the following statements **about your interaction with Alexa.**

| | 1 (116) | 2 (117) | 3 (118) | 4 (119) | 5 (120) | 6 (121) | 7 (122) | 8 (123) | 9 (124) | 10 (125) |
|---|---|---|---|---|---|---|---|---|---|---|
| Alexa was sensitive to what I was saying. (80) | ○ | ○ | ○ | ○ | ○ | ○ | ○ | ○ | ○ | ○ |
| Alexa seemed to understand what I said. (81) | ○ | ○ | ○ | ○ | ○ | ○ | ○ | ○ | ○ | ○ |
| Alexa seemed to listen to me for more than just spoken words. (82) | ○ | ○ | ○ | ○ | ○ | ○ | ○ | ○ | ○ | ○ |
| Alexa assured me that she got what I said. (83) | ○ | ○ | ○ | ○ | ○ | ○ | ○ | ○ | ○ | ○ |
| Alexa delivered a sense of agreement for what I was saying when appropriate. (84) | ○ | ○ | ○ | ○ | ○ | ○ | ○ | ○ | ○ | ○ |
| Alexa kept track of points I made. (85) | ○ | ○ | ○ | ○ | ○ | ○ | ○ | ○ | ○ | ○ |
| Alexa assured me that she was receptive to my ideas. (86) | ○ | ○ | ○ | ○ | ○ | ○ | ○ | ○ | ○ | ○ |
| Alexa assured me that I was listening by using verbal or nonverbal acknowledgments. (87) | ○ | ○ | ○ | ○ | ○ | ○ | ○ | ○ | ○ | ○ |

**Attitudes towards Alexa, measure by Kalyanaraman, S., & Sundar, S., 2006**

Please continue sharing your thoughts about your interaction with Alexa.
On the scale of 1 (Describes the Alexa Skill Very Poorly) to 10 (Describes the Alexa Skill Very

Well), how well do the following adjectives represent the **<u>Alexa Skill you used to interact with her?</u>**

| | 1 (22) | 2 (23) | 3 (24) | 4 (25) | 5 (26) | 6 (27) | 7 (28) | 8 (29) | 9 (30) | 10 (31) |
|---|---|---|---|---|---|---|---|---|---|---|
| Organized (14) | | | | | | | | | | |
| Good (15) | | | | | | | | | | |
| Useful (16) | | | | | | | | | | |
| Favorable (17) | | | | | | | | | | |
| Unique (18) | | | | | | | | | | |
| High quality (19) | | | | | | | | | | |
| User-friendly (20) | | | | | | | | | | |
| Exciting (21) | | | | | | | | | | |
| Stimulating (22) | | | | | | | | | | |
| Cool (23) | | | | | | | | | | |
| Interesting (24) | | | | | | | | | | |
| Coherent (25) | | | | | | | | | | |
| Pleasant (26) | | | | | | | | | | |
| Confusing (27) | | | | | | | | | | |
| Sophisticated (28) | | | | | | | | | | |
| Likable (29) | | | | | | | | | | |

| | | | | | | | | | | |
|---|---|---|---|---|---|---|---|---|---|---|
| Attractive (30) | ○ | ○ | ○ | ○ | ○ | ○ | ○ | ○ | ○ | ○ |
| Entertaining (31) | ○ | ○ | ○ | ○ | ○ | ○ | ○ | ○ | ○ | ○ |
| Appealing (32) | ○ | ○ | ○ | ○ | ○ | ○ | ○ | ○ | ○ | ○ |
| Intelligent (33) | ○ | ○ | ○ | ○ | ○ | ○ | ○ | ○ | ○ | ○ |
| Smart (34) | ○ | ○ | ○ | ○ | ○ | ○ | ○ | ○ | ○ | ○ |

**Post- study emotional survey, PANAS measures by Watson et al., 1988.**

On the scale of 1 (Not at All) to 10 (Very Much), how well do the following adjectives represent **how you feel at the moment**?

| | 1 (221) | 2 (222) | 3 (223) | 4 (224) | 5 (225) | 6 (226) | 7 (227) | 8 (228) | 9 (229) | 10 (230) |
|---|---|---|---|---|---|---|---|---|---|---|
| Enthusiastic (231) | ○ | ○ | ○ | ○ | ○ | ○ | ○ | ○ | ○ | ○ |
| Sad (232) | ○ | ○ | ○ | ○ | ○ | ○ | ○ | ○ | ○ | ○ |
| Content (233) | ○ | ○ | ○ | ○ | ○ | ○ | ○ | ○ | ○ | ○ |
| Embarrassed (234) | ○ | ○ | ○ | ○ | ○ | ○ | ○ | ○ | ○ | ○ |
| Nervous (235) | ○ | ○ | ○ | ○ | ○ | ○ | ○ | ○ | ○ | ○ |
| Angry (236) | ○ | ○ | ○ | ○ | ○ | ○ | ○ | ○ | ○ | ○ |
| Calm (237) | ○ | ○ | ○ | ○ | ○ | ○ | ○ | ○ | ○ | ○ |
| Anxious (238) | ○ | ○ | ○ | ○ | ○ | ○ | ○ | ○ | ○ | ○ |
| Happy (239) | ○ | ○ | ○ | ○ | ○ | ○ | ○ | ○ | ○ | ○ |
| Active (240) | ○ | ○ | ○ | ○ | ○ | ○ | ○ | ○ | ○ | ○ |

## REFERENCES


Gearhart, C. C., & Bodie, G. D. (2011). Active-empathic listening as a general social skill: Evidence from bivariate and canonical correlations. *Communication Reports*, *24*(2), 86-98.

Kalyanaraman, S., & Sundar, S. S. (2006). The psychological appeal of personalized content in web portals: does customization affect attitudes and behavior?. Journal of Communication, 56(1), 110-132.

Stiles, W. B., Barkham, M., Twigg, E., Mellor-Clark, J., & Cooper, M. (2006). Effectiveness of cognitive-behavioural, person-centred and psychodynamic therapies as practised in UK National Health Service settings. *Psychological medicine*, *36*(4), 555-566.

Watson, D., Clark, L. A., & Tellegen, A. (1988). Development and validation of brief measures of positive and negative affect: the PANAS scales. *Journal of personality and social psychology*, *54*(6), 1063.
